# Supplementary material for: Dissipation of Quasiclassical Turbulence in Superfluid $^4$He
Source: arXiv:1509.00813 ancillary file (2015-09-02)
Supplement: Supplementary file 1 [file PRL_SupplMatt_v9b.pdf]

# Supplemental Material: Quantitative Characterization of Observations

D. E. Zmeev
*School of Physics and Astronomy, The University of Manchester, Manchester M13 9PL, UK and Department of Physics, Lancaster University, Lancaster LA1 4YB, UK*

P. M. Walmsley and A. I. Golov
*School of Physics and Astronomy, The University of Manchester, Manchester M13 9PL, UK*

P. V. E. McClintock and S. N. Fisher*
*Department of Physics, Lancaster University, Lancaster LA1 4YB, UK*

W. F. Vinen
*School of Physics and Astronomy, University of Birmingham, Birmingham B15 2TT, UK*

(Dated: September 2, 2015)

PACS numbers: 47.80.Jk, 67.25.dk, 47.27.-i

## I. DETECTOR OF VORTEX LINES

The vortex line detector had two parts, which were fitted into the identical openings in the opposite vertical walls of the channel: the injector and collector assemblies. The injector consisted of a sharp tungsten tip [1] with a 92 % open tungsten grid in front of it. The collector was a brass disk with the same type of grid in front of it. By applying pulses of high voltage (400–600 V, 0.1 s long) to the injector tip, we produced current pulses (typically, 0.1 s long and of $I \lesssim 300$ pA in magnitude). In liquid helium, excess electrons form microscopic bubbles. At temperatures below 0.7 K they are attached to quantized vortex rings, thus forming charged vortex rings (CVRs). Both CVRs and bare electron bubbles, while moving in the vicinity of a vortex line, either change their trajectory or become trapped on the vortex lines. Hence, by measuring the attenuation of the magnitude of the peak of electric current arriving at the collector,

$$\gamma(L) = \ln \frac{I(0)}{I(L)}, \tag{1}$$

we could characterize the vortex tangle in the experimental volume.

Large-scale polarization (rotation) of the vortex tangle causes a sideway deflection of the beam of CVRs via the Coriolis effect. In the vortex detector, the guiding electric field could be made either converging (by grounding the injector grid while applying positive potential to the collector grid, typically +30 V) or diverging (by grounding the collector grid while applying negative potential to the injector grid, typically −60 V). The former assures that all injected CVRs end up within the collector disk; a small deflection of the beam off axis causing no change in the collector current. The latter, on the other hand, widens the beam of the CVRs beyond the diameter of the collector; by positioning the injector slightly off the vertical symmetry plane, we hence had a different response of the total collector current to small sideways deflections of the ions. We thus could use the detector in two regimes: (i) vortex line density meter ($\mathcal{L}$-meter) with converging field; (ii) detector of the vertical polarization of vorticity (P-detector) with diverging field. In both regimes, the detector was calibrated in steady rotation at fixed values of the angular velocity $\Omega$, when the experimetal volume is filled with an array of rectilinear vortices of the equilibrium density $\mathcal{L} = 2\Omega/\kappa$.

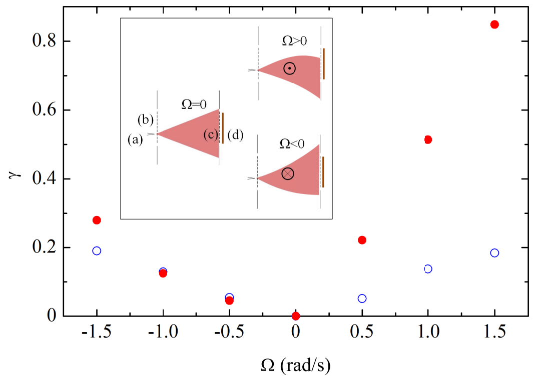


FIG. 1: Calibration of the vortex detector in the $\mathcal{L}$-meter regime (open circles) and P-detector regime (filled circles) in steady rotation. Inset shows a sketch (view from above) of the P-detector: the beam of CVRs is deflected either towards or away from the collector depending on the sense of rotation. Parts of the vortex detector: (a) tungsten tip, (b) injector grid, (c) collector grid, (d) collector.

In the P-detector regime, the current attenuation, $\gamma$, responded differently to opposite senses of rotation: $\gamma(\Omega) \neq \gamma(-\Omega)$, because the centre of the wide beam of CVRs was deflected either towards or away from the collector, as illustrated in the inset of Fig. 1. More pre-

*Deceased 4 January 2015.

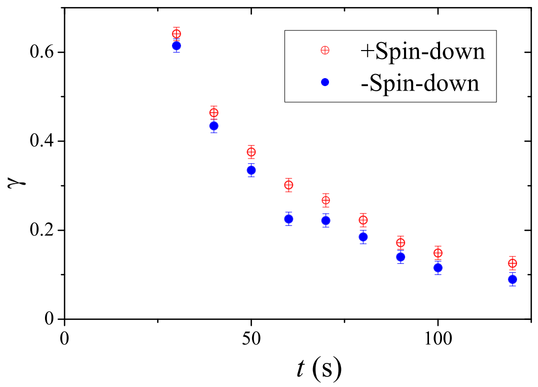


FIG. 2: The relative attenuation $\gamma$ of the collector current as function of time $t$ after an impulsive spin-down to rest from angular velocity $+1.5\,\mathrm{rad\,s^{-1}}$ and $-1.5\,\mathrm{rad\,s^{-1}}$. Diverging electrical field (P-detector). Temperature 80 mK.

cisely, $\gamma(\Omega) > \gamma(-\Omega)$ for $\Omega > 0$, as filled circles in Fig. 1 show. The P-detector, therefore, could be used to detect the sign of the vertical polarization of the vortex tangle. Our experiments at $T < 0.5\,\mathrm{K}$ reveal that the P-detector can distinguish between spin-down turbulence produced from the initial states with $\Omega = +1.5\,\mathrm{rad\,s^{-1}}$ and $\Omega = -1.5\,\mathrm{rad\,s^{-1}}$ (Fig. 1). Moreover, turbulence generated from the state with a positive $\Omega$ is characterized by a greater value of $\gamma$ compared to the state produced from $\Omega < 0$, as is the case in steady rotation (Fig. 1), when vertical polarization is the highest. Thus memory about the initial state in spin-down turbulence is retained down to late times of turbulence decay – presumably in the form of a slowly-rotating central core, weakly interacting with the turbulence near the walls.

The difference between $\gamma(t)$ after spin-down from $+1.5\,\mathrm{rad\,s^{-1}}$ and $-1.5\,\mathrm{rad\,s^{-1}}$ (as shown in Fig. 2, $T = 80\,\mathrm{mK}$) is roughly constant, $\gamma_+ - \gamma_- = 0.04 \pm 0.015$, for $30\,\mathrm{s} \leq t \leq 120\,\mathrm{s}$. Using the interpolation $|\Delta\gamma| \approx 0.4\,\mathrm{rad\,s^{-1}}|\Omega|$ at small $\Omega$ from the experimental data in Fig. 1 and assuming that the contributions to $\gamma \ll 1$ from the scattering of CVRs off vortex lines and from the deflection of the beam of CVRs by the Coriolis force are additive, we estimate the residual angular velocity of the central rotating vortex tangle at late time $30\,\mathrm{s} \leq t \leq 120\,\mathrm{s}$ as $\Omega_0 \sim 0.1\,\mathrm{rad\,s^{-1}}$ for $T = 80\,\mathrm{mK}$. The contribution from the polarized component of this tangle, $2\Omega_0/\kappa \sim 200\,\mathrm{cm^{-2}}$ is negligible compared to the mean $\mathcal{L}(t) \geq 1000\,\mathrm{cm^{-2}}$ at all times studied.

In the $\mathcal{L}$-meter regime, the electric current attenuation did not depend on the sense of rotation, $\gamma(\Omega) = \gamma(-\Omega)$ (open circles in Fig. 1), and the vortex line density is given by

$$\mathcal{L} = \gamma\sigma^{-1}d_h^{-1}, \tag{2}$$

where $\sigma$ is the mean scattering diameter for the given guiding field.

## II. CHARACTERIZATION OF INITIAL FLOWS

An important feature of well-developed turbulence is a wide range of length scales between which an inertial cascade is operating: from the integral length $\ell_0$ (from which the energy flux emerges) to the much smaller cut-off length (such as the Kolmogorov length $\eta$ in classical HIT, at which this energy of flow is converted into heat). To characterize each flow that generated turbulence at $t = 0$, we will estimate (see Table I and comments below) the integral length $\ell_0$, the integral Reynolds number

$$Re = \frac{\ell_0 u_0}{\nu'} \tag{3}$$

(where $u_0$ is the relative superfluid velocity at the integral scale and $\nu'$ is the effective kinematic viscosity) and the Kolmogorov length

$$\eta = \ell_0 Re^{-3/4}. \tag{4}$$

In the high-temperature regime, $T \gtrsim 1\,\mathrm{K}$, when the large-scale flows of the superfluid and normal components are coupled through the mutual friction, the effective kinematic viscosity is expected to be $\nu' \sim \mu_n/\rho \approx 1 \times 10^{-4}\,\mathrm{cm^2 s^{-1}}$ [2, 3], where $\mu_n$ is the dynamic viscosity of the normal component and $\rho$ is the total density of the coupled components. At lower temperatures, the viscosity of the normal component increases while the mutual friction decreases; as a result, the fluids decouple, and the dissipation in the superfluid component is controlled by the mutual friction (at intermediate temperatures only) and interactions between individual vortex lines (such as vortex reconnections and Kelvin wave cascade). As we show below, in the low-temperature limit, $\nu' \sim 1 \times 10^{-4}\,\mathrm{cm^2 s^{-1}}$ as well. We thus use this value for all regimes.

In QT, the lowest length scale of classical-like superfluid spectrum cannot be smaller than the mean intervortex separation $\ell_q = \mathcal{L}^{-1/2}$, which becomes the effective cut-off length of the classical cascade. We will hence estimate it at $t = 30\,\mathrm{s}$ (i. e. after the transient when the turbulence began its quasi-steady-state decay), and will also express the resulting inertial range in terms of the equivalent 'quantum Reynolds number' (see Table II),

$$Re_q = \left(\frac{\ell_0}{\ell_q}\right)^{4/3}, \tag{5}$$

obtained after substituting $\eta$ for $\ell_q$ in (4).

**Impulsive spin-down** from $\Omega_0 = 1.5\,\mathrm{rad\,s^{-1}}$ to rest results in $\ell_0 \sim d_h = 1.8\,\mathrm{cm}$, $u_0 \sim d_h\Omega_0 = 2.7\,\mathrm{cm\,s^{-1}}$. For the vortex line densities at the end of the initial transient (at $t \sim 10\,\mathrm{s}$), $\mathcal{L} = 7 \times 10^4\,\mathrm{cm^{-2}}$ at $T = 0.08\,\mathrm{K}$ and $\mathcal{L} = 7 \times 10^3\,\mathrm{cm^{-2}}$ at $T = 1.6\,\mathrm{K}$. As shown in [9], the initial transient, during which the initially rigidly-rotating flow breaks in several smaller eddies (presumably, Taylor vortices), lasts for $\sim 30\Omega_0^{-1}$, after which the decay follows $\mathcal{L} \propto t^{-3/2}$ indicating that the flow pattern has reached some statistical steady-state.

**Grid turbulence** is generated on the scale of mesh size [4], $\ell_0 = m_g$ (either 0.075 cm or 0.3 cm in our experiments) with the relevant velocity $u_0 = v_g$. During the transient process, the integral length increases until it is saturated by the channel size, $\ell_0 = d$, and stays constant afterwards. The saturation time has been measured in a channel with $d = 1$ cm for a range of $Re$ between $2 \times 10^3$ and $2 \times 10^5$ and was found to follow $t_{sat} \sim 4 \times 10^{-4} Re^{-1}$ s independent of temperature in the range 1.3 K – 1.95 K [5]. Even for our smallest $Re \sim 7 \times 10^3$ (for $v_m = 9\,\mathrm{cm\,s^{-1}}$, $m_g = 0.075$ cm) this corresponds to $t_{sat} \sim 6$ s, much shorter than the decay times $t$ between 30 s and 200 s, used for analysis. At the end of this transient, the integral length is $\ell_0 \approx (d_h + d_v)/2 = 1.75$ cm; with the initial $\mathcal{L} = 2.2 \times 10^4\,\mathrm{cm}^{-2}$.

**Ion-jet turbulence** was generated after 100 s of running the current of $\sim 0.7$ nA through the voltage $\sim 500$ V from injector tip to its grid; this current entrains the superfluid component resulting in the large-scale flow from injector to collector surrounded by backflow. The low bound on the velocity in the jet, $u_0 \gtrsim d_h/\tau_j \sim 0.6\,\mathrm{cm\,s^{-1}}$, can be estimated from the time of arrival at the collector, $\tau_j \sim 3$ s, of the first charged tangled vortices after starting the injection. The relevant integral length scale is $\ell_0 = d_v/2 = 0.85$ cm. Upon stopping injection and after the transient of several seconds, the values of decaying $\mathcal{L}(t)$ were virtually identical to those for the grid turbulence; we hence believe that the memory of the initial flow was lost at this stage, and both $\ell_0 = d$ and $\ell_q(t)$ are the same for both types of turbulence.

TABLE I: Parameters of flow as generated at $t = 0$

| Type of flow | $u_0$ | $\ell_0$ | $Re$ | $\eta$ |
|---|---|---|---|---|
| Sp-dn (1.5 rad $\mathrm{s^{-1}}$) | 2.7 cm $\mathrm{s^{-1}}$ | 1.8 cm | $5 \times 10^4$ | 5 $\mu$ |
| Grid (3 mm) | 15 cm $\mathrm{s^{-1}}$ | 0.3 cm | $5 \times 10^4$ | 1 $\mu$ |
| Ion jet (0.08 K) | > 1.8 cm $\mathrm{s^{-1}}$ | 0.85 cm | $> 1.5 \times 10^4$ | < 6 $\mu$ |
| Ion jet (1.6 K) | > 0.5 cm $\mathrm{s^{-1}}$ | 0.85 cm | $> 4 \times 10^3$ | < 16 $\mu$ |

TABLE II: Parameters at $t = 30$ s ($\ell_0 = 1.75$ cm for all)

| Type of flow | $\mathcal{L}_0$ | $\ell_q$ | $Re_q$ |
|---|---|---|---|
| Sp-dn (1.5 rad $\mathrm{s^{-1}}$, 0.08 K) | $7.7 \times 10^3\,\mathrm{cm^{-2}}$ | 110 $\mu$ | 820 |
| Grid or ion jet (0.08 K) | $3.7 \times 10^3\,\mathrm{cm^{-2}}$ | 170 $\mu$ | 500 |
| Any but at 1.6 K | $1.1 \times 10^3\,\mathrm{cm^{-2}}$ | 300 $\mu$ | 230 |

## III. ANALYSIS OF DECAYING $\mathcal{L}(t)$ USING THE APPROACH OF STALP *ET AL.* [6]

Stalp *et al.* [6] were the first to recognize that the $\mathcal{L} \propto t^{-3/2}$ dependence during free decay could be due to the saturation of the size of the energy-containing eddy by the container size. They introduced a method of interpreting the prefactor $A$ in terms of the value of $\zeta$ for HIQT. Since then this method has also been used by several groups [7–9]. It assumes that wall-bounded turbulence can be described by a single energy spectrum $E_k$ in the space of wavenumbers $k$. For $k > k_1$ (where $k_1 = 2\pi/d$ in [6]), this spectrum is taken to be equal to the Kolmogorov spectrum for HIT [12–14],

$$E_k = C\epsilon^{2/3}k^{-5/3} \tag{6}$$

(here $\epsilon = -\dot{\mathcal{E}}$ is the energy flux and $C \approx 1.5$ is the Kolmogorov constant), while for $k < k_1$, $E_k = 0$, because modes of size greater than the container do not exist. The total energy per unit volume is thus

$$\mathcal{E} \approx \int_{k_1}^{\infty} E_k dk = \frac{3}{2} C\epsilon^{2/3} k_1^{-2/3}, \tag{7}$$

and its rate of change during a quasi-steady decay is

$$\dot{\mathcal{E}} = -\epsilon = -(3C)^3 k_1^{-2} t^{-3} \tag{8}$$

at late time $t$. Equating this with Eq. 1 from the main Letter, we arrive at

$$\mathcal{L}(t) = (3C)^{3/2} \zeta^{-1/2} k_1^{-1} (\kappa t)^{-3/2}. \tag{9}$$

In other words, this model has just one free parameter, $k_1$, which depends on the container size and, perhaps, boundary conditions (BC). The lifetime of the eddy is kept equal to Kolmogorov's value for HIT (it is determined by the Kolmogorov constant $C$).

In order to make quantitative comparison of the rates of decay obtained in different experiments, we applied this one-parameter approach, Eq. 9 to our data $\mathcal{L} \propto t^{-3/2}$ from Fig. 3 of the main paper, with an appropriate choice of the value of the cut-off wavenumber $k_1$ that should

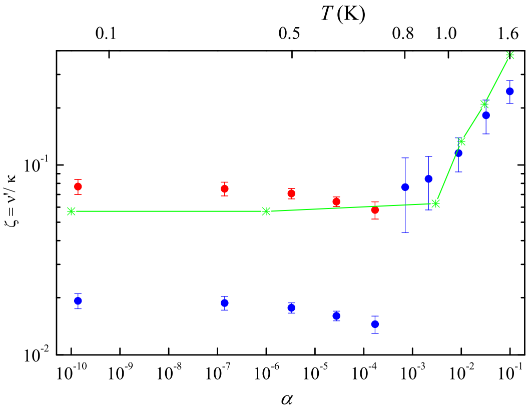


FIG. 3: Effective viscosity $\zeta = \nu'/\kappa$ vs. mutual friction parameter $\alpha(T)$ for grid turbulence (circles, see text). Green asterisks show the values of $\zeta$ for the decay of random tangles simulated numerically for different $\alpha$ [10] (the value $\zeta = 0.057$, plotted here at $\alpha = 10^{-10}$ and $\alpha = 10^{-6}$, was actually computed for $\alpha = 0$).

depend on the BC. Namely, for no-slip BC, one would expect $\lambda = d$, i. e. $k_1 = 2\pi/d$ (as was used by [6] while for slip BC, $\lambda = 2d$, i. e. $k_1 = 2\pi/2d = \pi/d$.

In Fig. 3 we plot the resulting values of $\zeta(\alpha)$ for grid turbulence. The blue symbols show the values of $\zeta$ obtained with $k_1 = 2\pi/d$, while the red ones, for $T \leq 0.8\,\mathrm{K}$ only, correspond to the values of $\zeta$ obtained using $k_1 = \pi/d$ (suitable for the slip BC at low temperatures). With the latter choice, the discontinuous drop in apparent data has vanished, and the dependence $\zeta(T)$ becomes smooth. Furthermore, it is close to the values $\zeta(0) = 0.08$ measured experimentally [15] and $\zeta(0) = 0.06$–$0.10$ calculated numerically [10, 11] (Fig. 3) for Vinen QT.

Unfortunately, several assumptions of the above approach are unrealistic. First of all, the description in terms of a unique $k$-spectrum while the system is strongly spatially-inhomogeneous (for instance, due to a particular shape of the container, or to the presence of a turbulent boundary layer) cannot be applied. But even if a one-for-all $k$-spectrum could be used, the Kolmogorov spectrum, Eq. 6, [12–14] was derived for wavenumbers $k$ far away from both those for forcing and dissipation. Hence, it is not expected to apply near the cut-off wavenumber $k_1$, and there is no reason why the total energy and its flux should be described by Eq. 7 and Eq. 8. We thus conclude that Eq. 9 can only yield the prefactor $A$ correct to an order of magnitude. Any numerical agreement must be purely accidental.


[1] A. Golov and H. Ishimoto, J. Low Temp. Phys. **113**, 957 (1998).

[2] W. F. Vinen, Phys. Rev. B **61**, 1410 (2000).

[3] W. F. Vinen and J. J. Niemela, J. Low Temp. Phys. **128**, 167 (2002).

[4] The presence of gaps $\sim 0.1\,\mathrm{cm}$ between the sides of the grid and the walls of the channel might complicate the flow (for instance, by generating an eddy at the scale of channel size $\sim d$ if the gap is uneven); however, our experimental observation that the decaying datasets $\mathcal{L}(t)$ were virtually identical for grids with different mesh sises $m_g$ (both smaller and larger than the gap) indicate that this was insignificant.

[5] L. Skrbek, J. J. Niemela, and R. J. Donnelly, Phys. Rev. Lett. **85**, 2973 (2000).

[6] S. R. Stalp, L. Skrbek, and R. J. Donnelly, Phys. Rev. Lett. **82**, 4831 (1999).

[7] S. R. Stalp , J. J. Niemela, W. F. Vinen, and R. J. Donnelly, Phys. Fluids **14**, 1377 (2002).

[8] D. I. Bradley *et al.*, Phys. Rev. Lett. **96**, 035301 (2006).

[9] P. M. Walmsley, A. I. Golov, H. E. Hall, A. A. Levchenko, and W. F. Vinen, Phys. Rev. Lett. **99**, 265302 (2007).

[10] M. Tsubota, T. Araki, and S. K. Nemirovskii, Phys. Rev. B **62**, 11751 (2000).

[11] L. Kondaurova, V. Lvov, A. Pomyalov, and I. Procaccia, Phys. Rev. B **90**, 094501 (2014).

[12] A. N. Kolmogorov, Dokl. Akad. Nauk. SSSR **32**, 19 (1941); reprinted in Proc. Roy. Soc. A **434**, 15 (1991).

[13] U. Frisch. Turbulence: The Legacy of A. N. Kolmogorov. Cambridge University Press, 1995.

[14] G. K. Batchelor. The Theory of Homogeneous Turbulence. Cambridge University Press, 1953.

[15] P. M. Walmsley and A. I. Golov, Phys. Rev. Lett. **100**, 245301 (2008).
